# Supplementary material for: DSWAM: A Dual-System World Action Foundation Model for Fine-Grained Robot Manipulation
Source: arXiv:2607.04927 source file (2026-07-06)
Supplement: Supplementary file 1 [file supplementary.tex]

\setcounter{figure}{0}
\setcounter{table}{0}

\section{Experiment}
\label{sec:appendix_experiment}

Table~\ref{tab:robotwin_full} reports per-task success rates on RoboTwin 2.0 under the clean and randomized settings. Motus and Fast-WAM are reported under both settings, while DSWAM is reported under the clean setting.

\begin{table}[t]
\centering
\caption{\raggedright \textit{Evaluation on RoboTwin 2.0 Simulation Benchmark}. Success rates are reported under clean and randomized settings across 50 bimanual manipulation tasks. Fast-WAM denotes the full model reported as Fast-WAM (Ours). DSWAM results are reported under the clean setting.}
\label{tab:robotwin_full}
\setlength{\tabcolsep}{3.0pt}
\resizebox{\textwidth}{!}{%
\begin{tabular}{l cc cc cc cc cc cc cc c}
\toprule
\multirow{2}{*}{\textbf{Simulation Task}} &
\multicolumn{2}{c}{$\pi_0$} & \multicolumn{2}{c}{$\pi_{0.5}$} & \multicolumn{2}{c}{X-VLA} & \multicolumn{2}{c}{LingBot-VLA} & \multicolumn{2}{c}{DeMaVLA} & \multicolumn{2}{c}{Motus} & \multicolumn{2}{c}{Fast-WAM} & \multicolumn{1}{c}{DSWAM} \\
\cmidrule(lr){2-3} \cmidrule(lr){4-5} \cmidrule(lr){6-7} \cmidrule(lr){8-9} \cmidrule(lr){10-11} \cmidrule(lr){12-13} \cmidrule(lr){14-15} \cmidrule(lr){16-16}
 & Clean & Rand. & Clean & Rand. & Clean & Rand. & Clean & Rand. & Clean & Rand. & Clean & Rand. & Clean & Rand. & Clean \\
\midrule
\textit{Adjust Bottle} & 99\% & 95\% & 100\% & 99\% & 100\% & 99\% & 100\% & 100\% & 99\% & 100\% & 89\% & 93\% & 100\% & 100\% & 100\% \\
\textit{Beat Block Hammer} & 79\% & 84\% & 96\% & 93\% & 92\% & 88\% & 87\% & 91\% & 79\% & 85\% & 95\% & 88\% & 99\% & 97\% & 100\% \\
\textit{Blocks Ranking RGB} & 80\% & 63\% & 92\% & 85\% & 83\% & 83\% & 92\% & 91\% & 95\% & 95\% & 99\% & 97\% & 100\% & 100\% & 100\% \\
\textit{Blocks Ranking Size} & 14\% & 5\% & 49\% & 26\% & 67\% & 74\% & 66\% & 73\% & 72\% & 68\% & 75\% & 63\% & 94\% & 98\% & 84\% \\
\textit{Click Alarmclock} & 77\% & 68\% & 98\% & 89\% & 99\% & 99\% & 93\% & 26\% & 98\% & 100\% & 100\% & 100\% & 100\% & 100\% & 100\% \\
\textit{Click Bell} & 71\% & 48\% & 99\% & 66\% & 100\% & 100\% & 32\% & 19\% & 96\% & 98\% & 100\% & 100\% & 100\% & 100\% & 100\% \\
\textit{Dump Bin Bigbin} & 88\% & 83\% & 92\% & 97\% & 79\% & 77\% & 97\% & 92\% & 91\% & 94\% & 95\% & 91\% & 97\% & 96\% & 88\% \\
\textit{Grab Roller} & 98\% & 94\% & 100\% & 100\% & 100\% & 100\% & 100\% & 99\% & 100\% & 100\% & 100\% & 100\% & 100\% & 100\% & 100\% \\
\textit{Handover Block} & 47\% & 31\% & 66\% & 57\% & 73\% & 37\% & 80\% & 83\% & 93\% & 83\% & 86\% & 73\% & 95\% & 81\% & 96\% \\
\textit{Handover Mic} & 97\% & 97\% & 98\% & 97\% & 0\% & 0\% & 94\% & 98\% & 95\% & 96\% & 78\% & 63\% & 99\% & 100\% & 96\% \\
\textit{Hanging Mug} & 14\% & 11\% & 18\% & 17\% & 23\% & 27\% & 32\% & 27\% & 46\% & 35\% & 38\% & 38\% & 58\% & 62\% & 61\% \\
\textit{Lift Pot} & 80\% & 72\% & 96\% & 85\% & 99\% & 100\% & 100\% & 99\% & 97\% & 94\% & 96\% & 99\% & 100\% & 100\% & 100\% \\
\textit{Move Can Pot} & 68\% & 48\% & 51\% & 55\% & 89\% & 86\% & 79\% & 84\% & 93\% & 79\% & 34\% & 74\% & 90\% & 88\% & 97\% \\
\textit{Move Pillbottle Pad} & 67\% & 46\% & 84\% & 61\% & 73\% & 71\% & 93\% & 94\% & 86\% & 86\% & 93\% & 96\% & 100\% & 99\% & 99\% \\
\textit{Move Playingcard Away} & 74\% & 65\% & 96\% & 84\% & 93\% & 98\% & 96\% & 99\% & 94\% & 90\% & 100\% & 96\% & 100\% & 100\% & 99\% \\
\textit{Move Stapler Pad} & 41\% & 24\% & 56\% & 42\% & 78\% & 73\% & 74\% & 49\% & 83\% & 76\% & 83\% & 85\% & 77\% & 64\% & 78\% \\
\textit{Open Laptop} & 71\% & 81\% & 90\% & 96\% & 93\% & 100\% & 96\% & 96\% & 98\% & 100\% & 95\% & 91\% & 98\% & 100\% & 99\% \\
\textit{Open Microwave} & 4\% & 32\% & 34\% & 77\% & 79\% & 71\% & 91\% & 75\% & 83\% & 72\% & 95\% & 91\% & 62\% & 45\% & 60\% \\
\textit{Pick Diverse Bottles} & 69\% & 31\% & 81\% & 71\% & 58\% & 36\% & 79\% & 86\% & 58\% & 75\% & 90\% & 91\% & 80\% & 85\% & 99\% \\
\textit{Pick Dual Bottles} & 59\% & 37\% & 93\% & 63\% & 47\% & 36\% & 82\% & 95\% & 89\% & 75\% & 96\% & 90\% & 100\% & 96\% & 100\% \\
\textit{Place A2B Left} & 43\% & 47\% & 87\% & 82\% & 48\% & 49\% & 86\% & 83\% & 92\% & 95\% & 88\% & 79\% & 95\% & 93\% & 94\% \\
\textit{Place A2B Right} & 39\% & 34\% & 87\% & 84\% & 36\% & 36\% & 74\% & 77\% & 90\% & 87\% & 91\% & 87\% & 93\% & 99\% & 93\% \\
\textit{Place Bread Basket} & 62\% & 46\% & 77\% & 64\% & 81\% & 71\% & 92\% & 93\% & 83\% & 84\% & 91\% & 94\% & 91\% & 93\% & 96\% \\
\textit{Place Bread Skillet} & 66\% & 49\% & 85\% & 66\% & 77\% & 67\% & 90\% & 89\% & 94\% & 83\% & 86\% & 83\% & 90\% & 93\% & 89\% \\
\textit{Place Burger Fries} & 81\% & 76\% & 94\% & 87\% & 94\% & 94\% & 95\% & 96\% & 96\% & 95\% & 98\% & 98\% & 96\% & 99\% & 96\% \\
\textit{Place Can Basket} & 55\% & 46\% & 62\% & 62\% & 49\% & 52\% & 68\% & 78\% & 87\% & 77\% & 81\% & 76\% & 71\% & 69\% & 64\% \\
\textit{Place Cans Plasticbox} & 63\% & 45\% & 94\% & 84\% & 97\% & 98\% & 97\% & 100\% & 89\% & 92\% & 98\% & 94\% & 99\% & 96\% & 100\% \\
\textit{Place Container Plate} & 97\% & 92\% & 99\% & 95\% & 97\% & 95\% & 99\% & 99\% & 96\% & 98\% & 98\% & 99\% & 96\% & 100\% & 98\% \\
\textit{Place Dual Shoes} & 59\% & 51\% & 75\% & 75\% & 79\% & 88\% & 80\% & 83\% & 96\% & 94\% & 93\% & 87\% & 94\% & 88\% & 85\% \\
\textit{Place Empty Cup} & 91\% & 85\% & 100\% & 99\% & 100\% & 98\% & 100\% & 100\% & 99\% & 99\% & 99\% & 98\% & 100\% & 100\% & 100\% \\
\textit{Place Fan} & 66\% & 71\% & 87\% & 85\% & 80\% & 75\% & 91\% & 79\% & 94\% & 91\% & 91\% & 87\% & 96\% & 96\% & 95\% \\
\textit{Place Mouse Pad} & 20\% & 20\% & 60\% & 39\% & 70\% & 70\% & 82\% & 78\% & 75\% & 78\% & 66\% & 68\% & 83\% & 89\% & 93\% \\
\textit{Place Object Basket} & 67\% & 70\% & 80\% & 76\% & 44\% & 39\% & 90\% & 91\% & 84\% & 66\% & 81\% & 87\% & 89\% & 88\% & 82\% \\
\textit{Place Object Scale} & 57\% & 52\% & 86\% & 80\% & 52\% & 74\% & 84\% & 90\% & 90\% & 89\% & 88\% & 85\% & 90\% & 97\% & 98\% \\
\textit{Place Object Stand} & 82\% & 68\% & 91\% & 85\% & 86\% & 88\% & 97\% & 93\% & 93\% & 92\% & 98\% & 97\% & 90\% & 94\% & 96\% \\
\textit{Place Phone Stand} & 49\% & 53\% & 81\% & 81\% & 88\% & 87\% & 92\% & 93\% & 95\% & 90\% & 87\% & 86\% & 97\% & 99\% & 95\% \\
\textit{Place Shoe} & 76\% & 76\% & 92\% & 93\% & 96\% & 95\% & 99\% & 94\% & 100\% & 100\% & 99\% & 97\% & 96\% & 99\% & 95\% \\
\textit{Press Stapler} & 44\% & 37\% & 87\% & 83\% & 92\% & 98\% & 90\% & 88\% & 96\% & 97\% & 93\% & 98\% & 90\% & 97\% & 87\% \\
\textit{Put Bottles Dustbin} & 65\% & 56\% & 84\% & 79\% & 74\% & 77\% & 88\% & 92\% & 88\% & 85\% & 81\% & 79\% & 95\% & 90\% & 92\% \\
\textit{Put Object Cabinet} & 73\% & 60\% & 80\% & 79\% & 46\% & 48\% & 92\% & 86\% & 92\% & 85\% & 88\% & 71\% & 94\% & 89\% & 92\% \\
\textit{Rotate QRcode} & 74\% & 70\% & 89\% & 87\% & 34\% & 33\% & 93\% & 84\% & 95\% & 86\% & 89\% & 73\% & 93\% & 89\% & 92\% \\
\textit{Scan Object} & 55\% & 42\% & 72\% & 65\% & 14\% & 36\% & 91\% & 97\% & 79\% & 83\% & 67\% & 66\% & 89\% & 92\% & 91\% \\
\textit{Shake Bottle Horizontally} & 98\% & 92\% & 99\% & 99\% & 100\% & 100\% & 100\% & 100\% & 100\% & 99\% & 100\% & 98\% & 100\% & 100\% & 100\% \\
\textit{Shake Bottle} & 94\% & 91\% & 99\% & 97\% & 99\% & 100\% & 99\% & 100\% & 100\% & 100\% & 100\% & 97\% & 100\% & 100\% & 99\% \\
\textit{Stack Blocks Three} & 72\% & 52\% & 91\% & 76\% & 6\% & 10\% & 92\% & 99\% & 97\% & 95\% & 91\% & 95\% & 95\% & 97\% & 99\% \\
\textit{Stack Blocks Two} & 93\% & 79\% & 97\% & 100\% & 92\% & 87\% & 100\% & 100\% & 100\% & 98\% & 100\% & 98\% & 100\% & 100\% & 100\% \\
\textit{Stack Bowls Three} & 77\% & 75\% & 77\% & 71\% & 76\% & 86\% & 72\% & 83\% & 83\% & 80\% & 79\% & 87\% & 80\% & 81\% & 83\% \\
\textit{Stack Bowls Two} & 94\% & 95\% & 95\% & 96\% & 96\% & 93\% & 92\% & 95\% & 98\% & 96\% & 98\% & 98\% & 92\% & 98\% & 93\% \\
\textit{Stamp Seal} & 46\% & 33\% & 79\% & 55\% & 76\% & 82\% & 76\% & 86\% & 77\% & 83\% & 93\% & 92\% & 90\% & 94\% & 89\% \\
\textit{Turn Switch} & 41\% & 42\% & 62\% & 54\% & 40\% & 61\% & 61\% & 65\% & 18\% & 41\% & 84\% & 78\% & 61\% & 59\% & 77\% \\
\midrule
\textbf{Average (\%)} & 65.92 & 58.40 & 82.74 & 76.76 & 72.80 & 72.84 & 86.50 & 85.34 & 88.42 & 86.78 & 88.66 & 87.02 & 91.88 & \textbf{91.78} & \textbf{92.38} \\
\bottomrule
\end{tabular}%
}
\vspace{-5pt}
\end{table}
